# Supplementary material for: UC Modelling and Security Analysis of the Estonian IVXV Internet Voting System
Source: arXiv:2109.01994 source file (2021-09-05)
Supplement: Supplementary file 1 [file additional.tex]

%! TEX encoding =UTF-8 Unicode
%! TEX root = mainArxiv.tex

%\subsubsection{Universally Composability (UC) Framework.}

We provide a review of the UC security framework. The current text is somewhat informal for clarity and brevity. Please refer to \cite{E:Canetti00} for full details.

%E:Canetti00,
Following Canetti’s framework \cite{FOCS:Canetti01}, a protocol is represented as interactive Turing machines (ITMs), each of which represents the program to be run by a participant. Protocols that securely carry out a given task are defined in three steps, as follows. First, the process of executing a protocol in an adversarial environment is formalized. Next, an ``ideal process'' for carrying out the task at hand is formalized. The parties have access to an ``ideal functionality,'' which is essentially an incorruptible ``trusted party'' that is programmed to capture the desired functionality of the task at hand. A protocol is said to securely realize an ideal functionality if the process of running the protocol amounts to ``emulating'' the ideal process for that ideal functionality. Below we overview the model of protocol execution (called the real-world model), the ideal process, and the notion of protocol emulation.
Meanwhile, each ITM has a session-identifier (SID) that describes which session (or, protocol instance) the ITM belongs to. It also has a party identifier (PID) that describes the role (or, participant identifier) of that ITM within the protocol instance. The pair (SID, PID) is guaranteed to be unique in the system.

\paragraph{The model for protocol execution.}
The model of computation consists of the parties running an instance of a protocol $\pi$, a network adversary $\Adv$ that controls the communication
among the parties, and an environment $\envZ$ that controls the inputs to the parties and sees
their outputs. The execution consists of a sequence of activations, where in each activation
a single participant (either $\envZ$, $\Adv$, or some other ITM) is activated, and may write on a tape of at most one other participant, subject to the rules below. Once the activation of a
participant is complete, the participant whose tape was written on is activated next.

Let $\ExA(\secp,z,r)$ denote the output of the environment $\envZ$ when interacting with parties running protocol $\pi$ on security parameter $\secp$, input $z$ and random input $r =r_{\envZ}, r_{\Adv}, r_1, r_2, \cdots$ as described above ($z$ and $r_{\envZ}$ for $\envZ$; $r_{\Adv}$ for $\Adv$, $r_i$ for party $\Pt_i$ ). Let $\ExA(k, z)$ denote the random variable describing $\ExA(k, z, r)$ when $r$ is uniformly chosen. Let $\ExA$ denote the ensemble $\{\ExA(k,z)\}_{k\in N,z\in\{0,1\}}^*$.

\paragraph{Ideal functionalities and ideal protocols.}
Security of protocols is defined via comparing the protocol execution to an ideal protocol for carrying out the task at hand. A key ingredient in the ideal protocol is the ideal functionality that captures the desired functionality, or the specification, of that task. The ideal functionality is modeled as another ITM (representing
a ``trusted party'') that interacts with the parties and the adversary. More specifically, in the ideal protocol for functionality $\ifunc$ all parties simply hand their inputs to an ITM instance running $\ifunc$.

\paragraph{Securely realizing an ideal functionality. }
We say that a protocol $\pi$ emulates protocol $\phi$ if for any network adversary $\Adv$ there exists an adversary (also known as simulator) $\Simu$ such that no environment $\envZ$, on any input, can tell with non-negligible probability whether it is interacting with $\Adv$ and parties running $\pi$, or it is interacting with S and parties running $\phi$. This means that, from the point of view of the environment, running protocol $\pi$ is ``just as good'' as interacting with $\phi$. We say that $\pi$ securely realizes an ideal functionality $\ifunc$ if it emulates the ideal protocol for $\ifunc$. More precise definitions follow. A distribution ensemble is called binary if it consists of distributions over $\{0, 1\}$.

\begin{definition}
 Let $\pi$ and $\phi$ be protocols, and $\ifunc$ be an ideal functionality. We say that $\pi$ UC-emulates $\phi$ if for any adversary $\Adv$ there exists an adversary $\Simu$ such that for any environment $\envZ$ that obeys the rules of interaction for UC security we have $\ExS\approx \ExA$. We say that $\pi$ UC-realizes  $\ifunc$ if $\pi$ UC-emulates the ideal protocol for functionality $\ifunc$.

\end{definition}

\begin{remark}[Hybrid protocols.]
Hybrid protocols are protocols where, in addition to communicating as usual as in the standard model of execution, the parties also have access to (multiple copies of) an ideal functionality. Hybrid protocols represent protocols that use idealizations of underlying primitives, or alternatively make trust assumptions on the underlying network.
They are also instrumental in stating the universal composition theorem. Specifically, in
an $\ifunc$-hybrid protocol (i.e., in a hybrid protocol with access to an ideal functionality $\ifunc$), the parties may give inputs to and receive outputs from an unbounded number of copies of $\ifunc$. The definition of a protocol securely realizing an ideal functionality is extended to hybrid protocols in the natural way.
\end{remark}
